# Supplementary material for: SelfSearch: Reward-Free Search for Self-Improving Agents
Source: arXiv:2609.37968 source file (2026-09-30)
Supplement: Supplementary file 1 [file additional_verified_tasks.tex]

\texttt{astropy\_\_astropy-7166} & \texttt{django\_\_django-11333} & \texttt{django\_\_django-13964} \\
\texttt{astropy\_\_astropy-7606} & \texttt{django\_\_django-11477} & \texttt{django\_\_django-14011} \\
\texttt{astropy\_\_astropy-8707} & \texttt{django\_\_django-11551} & \texttt{django\_\_django-14017} \\
\texttt{astropy\_\_astropy-8872} & \texttt{django\_\_django-11555} & \texttt{django\_\_django-14089} \\
\texttt{astropy\_\_astropy-12907} & \texttt{django\_\_django-11740} & \texttt{django\_\_django-14140} \\
\texttt{astropy\_\_astropy-13236} & \texttt{django\_\_django-12741} & \texttt{django\_\_django-14238} \\
\texttt{astropy\_\_astropy-13398} & \texttt{django\_\_django-12965} & \texttt{django\_\_django-14311} \\
\texttt{astropy\_\_astropy-14096} & \texttt{django\_\_django-13128} & \texttt{django\_\_django-14351} \\
\texttt{astropy\_\_astropy-14182} & \texttt{django\_\_django-13158} & \texttt{django\_\_django-14376} \\
\texttt{astropy\_\_astropy-14539} & \texttt{django\_\_django-13297} & \texttt{django\_\_django-14493} \\
\texttt{astropy\_\_astropy-14995} & \texttt{django\_\_django-13315} & \texttt{django\_\_django-14534} \\
\texttt{django\_\_django-11095} & \texttt{django\_\_django-13343} & \texttt{django\_\_django-14580} \\
\texttt{django\_\_django-11119} & \texttt{django\_\_django-13406} & \texttt{django\_\_django-14631} \\
\texttt{django\_\_django-11133} & \texttt{django\_\_django-13449} & \texttt{django\_\_django-14672} \\
\texttt{django\_\_django-11138} & \texttt{django\_\_django-13551} & \texttt{django\_\_django-14725} \\
\texttt{django\_\_django-11163} & \texttt{django\_\_django-13658} & \texttt{django\_\_django-14752} \\
\texttt{django\_\_django-11211} & \texttt{django\_\_django-13670} & \texttt{django\_\_django-14765} \\
\texttt{django\_\_django-11239} & \texttt{django\_\_django-13741} & \texttt{django\_\_django-14771} \\
\texttt{django\_\_django-11276} & \texttt{django\_\_django-13786} & \texttt{django\_\_django-14787} \\
\texttt{django\_\_django-11292} & \texttt{django\_\_django-13837} & \texttt{django\_\_django-14855} \\
